# Supplementary material for: GRaCE: Balancing Multiple Criteria to Achieve Stable, Collision-Free, and Functional Grasps
Source: arXiv:2309.08887 source file (2024-05-29)
Supplement: Supplementary file 1 [file appendix.tex]

\clearpage
\nobalance
\section*{Appendix}

\subsection{Event camera biases}
We tuned the hardware bias settings of Prophesee Onboard in order to minimize noise and latency, %\wcnote{Basically if we set some thresholds too high, a huge change is needed to trigger spikes and therefore spikes fire generally later.} 
while retaining a good amount of signal. Table \ref{tbl:biases} shows selected key biases using Prophesee's conventions; note that the parameter values are unitless. A  file containing the full set of biases is available online at \href{https://clear-nus.github.io/visuotactile/}{https://clear-nus.github.io/visuotactile/}.

\begin{table}[h]
\centering 
\caption{Prophesee Biases}
\label{tbl:biases}
\begin{tabular}{ccc}
 \hline 
 \hline 
   \textbf{Bias} & \textbf{Value} & \textbf{Remarks}  \\
  \hline
 bias\_fo & 1775 & Pixel low-pass cut-off frequency \\ 
 \hline
 bias\_hpf & 1800 & Pixel high-pass cut-off frequency \\
 \hline
 bias\_pr & 1550 & Controls photo-receptor \\
 \hline
 bias\_diff\_on & 435 & Sensitivity to positive change in luminosity \\
 \hline
 bias\_diff\_off & 198 & Sensitivity to negative change in luminosity \\
 \hline
 bias\_refr & 1500 & Pixel refractory period  \\
 \hline
 \hline 
\end{tabular}
\end{table}

\subsection{Handling Phase Shift}
%In our multi-modal setting, tactile events firing upon grasp onset necessarily correlates with a simultaneous decrease in vision events, since the gripper is settling to an equilibrium. 
Minimizing phase shift is critical, so that machine learning models can learn meaningful interactions between the different modalities. Our setup spanned across multiple machines, each having an individual Real Time Clock (RTC). We used \textit{chronyd} to sync our clocks to the Google Public NTP pool time servers. During data collection, for each machine, we logged the record-start time according to its own RTC, and thus were able to retrieve differences between the different RTCs and sync them accordingly during data pre-processing.

\subsection{Ground-truth Slip detection}

In our data collection procedure, rotational slip typically happened in the middle of a recording. In order to extract the relevant portion of the data when slip occurred, we first detected and annotated the slip onset. We attached OptiTrack markers on Panda's end-effector and the object, such that the OptiTrack was able to determine their poses. Fig. \ref{fig:optitrack} visualizes the OptiTrack data for a typical slipping data point. We annotated the OptiTrack frame $f_{lift}$ when the robot first lifted the object up using the following heuristic:
\[   
\frac{1}{120}\sum_{i=1}^{120} I(p_{z,j}>p_{z,i}) > 0.98 = 
     \begin{cases}
       \text{False} &\quad\text{}j = f_{lift} - 1\\
       \text{True} &\quad\text{}j \geq f_{lift} \\ 
     \end{cases}
\]
%We did not attempt to model OptiTrack noise since position and orientation can have non-trivial correlation. 
We checked when $p_z$ departed the empirical noise distribution within $f_{1,\dots,120}$ when the robot arm was stationary. 

%In my experience, for any marker detection algorithm for AR markers, there is correlation between positional error and orientation error. There is also correlation within position (px py pz), and also correlation within orientation (qx qy qz qw). I confidently assume this applies to OptiTrack too, even though I probably can't articulate this well verbally or in writing. Back then I thought it might be foolist to try and fit a statistical distribution on say p_z directly. Even if distribution fit is good, the context makes it wrong.

For object orientation, we computed the change in angle from at rest using $\theta_t \;=\; \cos^{-1}\bigl(2\langle q_0,q_t\rangle^2 -1\bigr)$, where $q_0$ is the quaternion orientation at rest. Similarly, we annotated the frame $f_{slip}$ when the object first rotates using the following heuristic:
\[   
\frac{1}{120}\sum_{i=1}^{120} I(\theta_j>\theta_i) > 0.98 = 
     \begin{cases}
       \text{False} &\quad\text{}j = f_{slip} - 1\\
       \text{True} &\quad\text{}j \geq f_{slip} \\ 
     \end{cases}
\]
We find that the time it takes for the object to rotate upon lifting was on average 0.03 seconds across all of the slipping data points. %This means that the object slips effectively immediately.

%I emphasized OptiTrack POV so far because, instead of end-effector moving up from OptiTrack POV, we can very well use other parts of the data, such as Panda's proprioceptive data in our rosbag, or the trajectory timestamps of distinct phases. The ones I mention so far may be subject to latency or phase shift issues, and so I decided that OptiTrack is the way to go.

\begin{figure} 
\centering
\includegraphics[width=1\columnwidth]{images/optitrack_plot_for_appendix.png}
\caption{(\textbf{Top}) $p_z$ of end-effector across time. As the robot arm lifts the object up, $p_z$ increases. (\textbf{Bottom}) $\theta_t$ (shortest angle in radians) computed between $q_t$ and $q_0$. This increases as the object slips. (\textbf{All}) The red vertical line indicates the point where $p_z$ increases significantly from at rest, and the blue vertical line indicates the point where $\theta_t$ increases significantly from at rest. The difference is 0.03 seconds for this data point.}
\label{fig:optitrack}
\end{figure}

\subsection{3D-Printed Parts}
We mounted the visual-tactile sensor components to the robot via 3D printed parts (Fig.\ref{fig:robotsetup}). There are three main 3D printed parts; a main holder (Fig.\ref{fig:main_holder}) to mount Intel RealSense D435, Prophesee Onboard and ACES encoder to the Franka Emika Panda arm, an enclosure for the ACES encoder (Fig.\ref{fig:second_holder}-a) and a coupler to mount the NeuTouch fingers onto Robotiq 2F-140 (Fig.\ref{fig:second_holder}-b).
All of the 3D printed parts for our project were printed using Acrylonitrile Butadiene Styrene (ABS) with layer thickness set to $0.2$ mm. We minimized total weight while maintaining structural integrity by maximizing the infills of only a select few components. All 3D components are available online at \href{https://clear-nus.github.io/visuotactile/}{https://clear-nus.github.io/visuotactile/}.

\begin{figure}
\centering
\begin{minipage}{0.90\columnwidth}
\centering
\includegraphics[width=0.80\columnwidth]{images/printed_parts/main_holder.pdf}
\caption{3D-printed main holder. This 3D assembly consists of 4 parts: (a) a semi-arc to secure main holder to the 7th link of the Panda arm (infill 99\%); (b) connector to attach sensors to the Panda (infill 99\%) (c) a base for mounting the enclosure of ACES encoder (infill 80\%); (d) a holder for the Intel RealSense D435 and Prophesee Onboard (infill 80\%).}
\label{fig:main_holder}
\end{minipage}\\
\vspace{0.5cm}
\begin{minipage}{0.95\columnwidth}
\centering
\includegraphics[width=0.80\columnwidth]{images/printed_parts/second_parts.pdf}
\caption{ (a) An enclosure for the ACES encoder (infill 65\%); (b) A coupler for NeuTouch (infill 99\%). }
\label{fig:second_holder}
\end{minipage}
%\vspace{15cm}
\end{figure}

\subsection{Container \& Weight Dataset Version 2.0}
Since the publication of this paper, we have collected a second larger version of the weight container dataset with 40 samples per class (Version 2). For this dataset, we used a slightly different version of the  NeuTouch, which was manufactured to be more physically robust. The objects order during data collection was also randomized to mitigate any possible drift.

We ran the VT-SNN on this dataset, with binning thresholds $S_{\min}=0$ for tactile, and $S_{\min}=1$ for vision. The obtained final accuracies are given in Table~\ref{tbl:classacc325_aug13data}. We also show early classification of the our models across time in Fig~\ref{fig:classtime_aug13data}. Overall, the findings are qualitatively similar to the previous dataset, i.e., the combined model still performs the best (albeit with a smaller improvement over vision). The weighted spike-count loss improves the overall performance of the models in the early phases of the classification. 

\begin{figure}
\centering
\includegraphics[width=0.80\columnwidth]{images/analysis/object_det_over_time_new_aug13.pdf}
% \caption{Container and weight classification accuracy over time. Lines show average test accuracy and shaded regions represent the standard deviations.  Vision-only classification results in higher early accuracy as visual spikes are obtained as the gripper is closing, and tactile events arise only upon contact with the object. Combining both vision and tactile event data via our VT-SNN results in significantly higher accuracy, compared to using each modality separately. }
\caption{Container and weight classification accuracy over time for Version 2 of the dataset.}

\label{fig:classtime_aug13data}
\end{figure}

\begin{table}
\centering 
\caption{Container \& Weight Classification (Entire Input Sequence): Average Accuracy with Standard Deviation in Brackets}
\label{tbl:classacc325_aug13data}
\begin{tabular}{l|ccc}
 \hline 
 \hline 
  \textbf{Model} & \textbf{Tactile} & \textbf{Vision} & \textbf{Combined} \\
  \hline
 SNN ($\mathcal{L}$) & 0.57 (0.055) & 0.74 (0.054)  & 0.78 (0.022)\\
  \hline
 SNN  ($\mathcal{L}_\omega$) & 0.55 (0.036) & 0.74 (0.058)  & 0.77 (0.018)\\
  \hline 
 ANN (MLP-GRU) & 0.46 (0.048) & 0.45 (0.048) & 0.47 (0.030)\\
   \hline 
 ANN (CNN-3D) & 0.67 (0.050) & 0.65 (0.015) & 0.69 (0.042) \\
 %ANN (CNN-GRU) & & & \\
%  \hline 
% EST \cite{Gehrig_2019_ICCV}  & 0.795 (0.029) & 0.820 (0.061) & -- \\
 \hline 
 \hline 
\end{tabular}
\end{table}

\subsection{Power Utilization and Latency Benchmarks}

We trained the multi-modal VT-SNN using the SLAYER framework for the task of rotational slip detection\footnote{Our benchmarking scripts for the GPU are made available in our code repository.}. The model and experimental setup is identical to rotational slip detection described in Section ~\ref{sec:slip}, with two changes:

\begin{enumerate}
    \item The Loihi neuron model is used in place of the SRM neuron model.
    \item The polarity of the vision output is discarded to reduce the vision input size to fit into a single core on the Loihi.
\end{enumerate}

Both models attain 100\% test accuracy, and produce identical results on the Loihi and the GPU. All benchmarks were obtained for the Loihi using NxSDK version 0.9.5 on a Nahuku 32 board, and on a Nvidia RTX 2080Ti GPU respectively.

\vspace{0.3em}
\noindent\textbf{Task.}
The model is tasked to perform 1000 forward passes, with a batch size of 1 on the GPU. The dataset of 1000 samples is obtained by repeating samples from our test set. Each sample consists of 0.15s of spike data, binned every 1ms into a 150 timesteps.

\vspace{0.3em}
\noindent\textbf{Latency.}
% On the GPU, the system clock on the CPU was used to capture the start ($t_{start}$) and end time ($t_{end}$) for model inference, and on the Loihi, we used the system clock on superhost. We compute the latency per timestep as $(t_{end} - t_{start}) \div 1000 \div 150$, dividing across 1000 samples, each with 150 timesteps.
On the GPU, the system clock on the CPU was used to capture the start ($t_{start}$) and end time ($t_{end}$) for model inference, and on the Loihi, we used the system clock on superhost. We compute the latency per timestep as $(t_{end} - t_{start}) / (1000 \times 150)$, dividing across 1000 samples, each with 150 timesteps.

\vspace{0.3em}
\noindent\textbf{Power Utilization.}
To obtain power utilization on the GPU, we adopt the approach in~\cite{blouw2018benchmarking} and used the NVIDIA System Management Interface, logging \texttt{(timestamp, power\_draw)} pairs at 200ms intervals with the utility. We extracted the power draw during the time spent, and averaged it to obtain the average power draw under load. To obtain the idle power draw of the GPU, we logged power usage on the GPU for 15 minutes with no processes running on the GPU, and averaged the power draw over the period.

We use the performance profiling tools available within NxSDK 0.9.5 to obtain the power utilization for the VT-SNN on the Loihi. Our model is small and occupies less than 1 chip on the 32-chip Nahuku 32 board. To obtain more accurate power measurements, we replicate the workload 32 times and report the results per-copy. The replicated workload occupies 594 neuromorphic cores and 5 x86 cores, with 624 neuromorphic cores powered for barrier synchronization.

For the first experiment, the data was passed directly to the models. The benchmark results are presented in Table~\ref{tbl:benchmark-exp1}. We observe that the model performed inference about 10x slower on the Loihi as compared to the GPU. This was due to the data being presented faster than real time. Here, the Loihi was bottlenecked by the speed of spike injection into the x86 cores. In a more practical setting, spike data would arrive at intervals of 1ms, and the Loihi would be able to process them as they arrive, while the GPU would have to accumulate data for the full 0.15s window before performing the forward pass.

\begin{table*}
\centering
\caption{Inference Speed and Power Utilization (Offline)}
\label{tbl:benchmark-exp1}
\begin{tabular}{cc|ccc|c|c|c}
 \hline 
 \hline
 \multicolumn{2}{c|}{Hardware} & \multicolumn{3}{c|}{Power ($mW$)} & \multirow{2}{*}{Latency per Timestep ($\mu s$)} & \multirow{2}{*}{Energy per Timestep ($\mu J$)} & \multirow{2}{*}{Energy-Delay Product (nJs)} \\
  { } & & Static & Dynamic & Total &  &  &  \\
 \hline 
\multirow{3}{*}{Loihi} & x86 cores & 0.19 & 21.1 & 21.3 & - & 0.14 & - \\
& neuron cores & 11.7 & 0.64 & 12.4 & - & 0.08 & - \\
& total & 11.9 & 21.7 & 33.7 & 231 & 0.22 & 51.8 \\
\hline
GPU & total & 3594 & 56296 & 59890 & 21 & 399 & 8431 \\
 \hline 
 \hline 
\end{tabular}
\end{table*}

\begin{table*}
\centering
\caption{Inference Speed and Power Utilization (Real-world Simulation)}
\label{tbl:benchmark-exp2}
\begin{tabular}{cc|ccc|c|c|c}
 \hline 
 \hline
 \multicolumn{2}{c|}{Hardware} & \multicolumn{3}{c|}{Power ($mW$)} & \multirow{2}{*}{Latency per Timestep ($\mu s$)} & \multirow{2}{*}{Energy per Timestep ($\mu J$)} & \multirow{2}{*}{Energy-Delay Product (nJs)} \\
  { } & & Static & Dynamic & Total &  &  &  \\
 \hline 
\multirow{3}{*}{Loihi} & x86 cores & 0.19 & 20.1 & 20.3 & - & 0.14 & - \\
& neuron cores & 11.9 & 0.15 & 12.1 & - & 0.08 & - \\
& total & 12.1 & 20.23 & 32.3 & 1039.9 & 0.22 & 224 \\
\hline
GPU & total & 3594 & 58336 & 61930 & 1045.6 & 412.9 & 431708 \\
 \hline 
 \hline 
\end{tabular}
\end{table*}

We then ran a second experiment that simulates accurately the real-world setting. The setup is identical to the first experiment, with two changes:

\begin{enumerate}
    \item The x86 cores are artificially slowed down to match the 1ms timestep duration of the data.
    \item An artificial delay of 0.15s is introduced to the dataset fetch for the GPU, to simulate waiting for the full window of data before it is able to perform inference.
\end{enumerate}

The results are presented in Table~\ref{tbl:benchmark-exp2}. We observe that the inference speeds on the GPU and Loihi are comparable in this scenario, but the Loihi consumes 1927x less power than the GPU. The Loihi's slightly faster inference speed is likely due to the chip being able to process the spikes as they arrive, while the GPU needs to wait for the full window of spiking data to arrive before performing inference. However, we note that the GPU remains more efficient for offline, batched processing of spiking data, and the latency difference would be further compounded by passing data in larger batch sizes to the GPU.

% \section{Handling phase shift}
